# Supplementary material for: AndroidLab: Training and Systematic Benchmarking of Android Autonomous Agents
Source: arXiv:2410.24024 source file (2024-11-04)
Supplement: Supplementary file 1 [file 5_limitation.tex]

\section*{Limitations}

\vpara{Limited Expandability of Evaluation Tasks.}
All evaluation tasks in our study are predefined and hardcoded. This means that if new evaluation tasks need to be added in the future, they must be individually and manually integrated, which is a time-consuming and not easily scalable process.

\vpara{Fixed Wait Time for Actions.}
In the action space, the model waits for a fixed period after selecting each action to allow the device to respond. However, this fixed waiting time does not account for the variability of response times across Android devices. Such variability can be attributed to several factors, including the device model, age, and user-specific configurations. Consequently, it is challenging to establish a universally applicable wait time for responses.

\vpara{Lack of Cross-Platform Capability.}
It is important to note that our evaluation framework is limited to the Android operating system and cannot be used to evaluate models operating on other systems, such as iOS or other device platforms. This limitation renders our framework applicable solely to a single platform.

\section*{Potential Risks}

\vpara{Risk Avoidance in Benchmark Design.} In the design of our benchmark, we have avoided potentially risky operations such as payments and sending messages. Additionally, our benchmark is tested on virtual machines without an internet connection, further preventing the actual execution of these operations. However, in real-world scenarios where agents are used, special attention should be paid to the correctness of such operations when the user provides these kinds of tasks. We plan to add sensitive operation protection in future systems, meaning these operations require explicit user consent before execution.

\vpara{Ensuring XML Quality for Apps.} The XML quality of certain apps might be poor, possibly loading too much or too little content. In actual deployment, it is essential to carefully inspect the XML quality of each app to ensure accurate usage.
